# Supplementary material for: Equivariant Transformer Networks
Source: arXiv:1901.11399 source file (2019-05-24)
Supplement: Supplementary file 2 [file supplementary-dataset.tex]

\section{Projective MNIST Dataset}
\label{appendix:projective-mnist}
