# Supplementary material for: Equivariant Transformer Networks
Source: arXiv:1901.11399 source file (2019-05-24)
Supplement: Supplementary file 4 [file supplementary-implementation.tex]

\section{Implementation Details}
\label{appendix:implementation}
