# Supplementary material for: Equivariant Transformer Networks
Source: arXiv:1901.11399 source file (2019-05-24)
Supplement: Supplementary file 5 [file supplementary-lie.tex]

\section{Background on Lie Groups}
\label{appendix:lie}
